# Supplementary material for: Adaptive Differentially Private Structural Entropy Minimization for Unsupervised Social Event Detection
Source: arXiv:2407.18274 source file (2024-07-23)
Supplement: Supplementary file 1 [file 7-appendix.tex]

% \clearpage
% \appendix

% \section{Split results of Event2012}
% \label{sec:SplitEvent2012}
% \begin{table}[!h]
%     \caption{Split results of Event2012}
%     \centering
%     \renewcommand\arraystretch{0.8}
%     \setlength{\tabcolsep}{1.5mm}
%     \resizebox{\linewidth}{!}{
%     \begin{tabular}{c||c c c c c c c}
%         \toprule
%         Blocks &$M_0$ &$M_1$ &$M_2$ &$M_3$ &$M_4$ &$M_5$ &$M_6$   \\
%         \hline
%         messages &20,254 &8,722 &1,491  &1,835  &2,010  &1,834  &1,276   \\
%         events &155 &41 &30  &33  &38  &30  &44    \\
%         \toprule

%         \toprule
%         Blocks &$M_7$ &$M_8$ &$M_9$ &$M_{10}$ &$M_{11}$ &$M_{12}$ &$M_{13}$   \\
%         \hline
%         messages &5,278  &1,560  &1,363  &1,096  &1,232  &3,237  &1,972      \\
%         events &57  &53  &38  &33 &30 & 42 &40    \\
%         \toprule

%         \toprule
%         Blocks &$M_{14}$ &$M_{15}$ &$M_{16}$ &$M_{17}$ &$M_{18}$ &$M_{19}$ &$M_{20}$ \\
%         \hline
%         messages &2,956  &2,549  &910  &2,676  &1,887  &1,399  &893 \\
%         events &43  &42  &27  &35  &32  &28  &34 \\
%         \toprule

%         \toprule
%         Blocks  &$M_{21}$\\
%         \hline
%         messages  &2,410\\
%         events  &32\\
%         \toprule
%     \end{tabular}}
% \label{s_event2012}
% \end{table}
% \vspace{-2mm}

% \section{Split results of Event2018}
% \label{sec:SplitEvent2018}
% \begin{table}[!h]
%     \caption{Split results of Event2018}
%     \renewcommand\arraystretch{0.8}
%     \setlength{\tabcolsep}{1.5mm}
%     \begin{tabular}{c||c c c c c c c}
%         \toprule
%         Blocks &$M_0$ &$M_1$ &$M_2$ &$M_3$ &$M_4$ &$M_5$ &$M_6$   \\
%         \hline
%         messages &14,328 &5,356 &3,186  &2,644 &3,179  &2,662  &4,200   \\
%         events &79 &22 &19  &15  &19  &27  &26    \\
%         \toprule

%         \toprule
%         Blocks &$M_7$ &$M_8$ &$M_9$ &$M_{10}$ &$M_{11}$ &$M_{12}$ &$M_{13}$   \\
%         \hline
%         messages &3,454  &2,257  &3,669  &2,385  &2,802  &2,927  &4,884      \\
%         events &23  &25  &31  &32 &31 & 29 &28    \\
%         \toprule

%         \toprule
%         Blocks &$M_{14}$ &$M_{15}$ &$M_{16}$  \\
%         \hline
%         messages &3,065  &2,411  &1,107   \\
%         events &26  &25  &14  & \\
%         \toprule
%     \end{tabular}
% \label{s_event2018}
% \end{table}
% \vspace{-2mm}


% \section{Hierarchical 2D SE Minimization.}
% \label{sec:Hierarchical0}

% \resizebox{\linewidth}{!}{
% \begin{algorithm}[!h]
%     \caption{Hierarchical 2D SE Minimization}
%     \label{alg:2D0}
%     \renewcommand{\algorithmicrequire}{\textbf{Input:}}
%     \renewcommand{\algorithmicensure}{\textbf{Output:}}
%     \begin{algorithmic}[1]
%         \REQUIRE a message graph $G = (V, E) $, sub-graph size $n$  %%input
%         \ENSURE event label set $P = \{p_1, \dots ,p_N\}$    %%output
        
%         \STATE $P$ $\leftarrow$ $(m|m \in V)$
%         \WHILE{\text{TRUE}}
%             \STATE {$P_s$} $\leftarrow$ consecutively remove the first min($n$, size of the remaining part of $P$) clusters from $P$ that form a set $P_s$
%             \FOR {each $P_s$ $\in$ $\{P_s\}$} 
%                 \STATE $V'$ $\leftarrow$ combine all the clusters in $P_s$
%                 \STATE $E'$ $\leftarrow$ {$e \in E$, both endpoints of $e \in V'$}
%                 \STATE $G$ $\leftarrow$ $(V', E')$
%                 \STATE $\mathcal{T'}$ $\leftarrow$ add a root tree node $ \lambda $
%                 \FOR {each $cluters C \in P_s$}
%                     \STATE Add a tree node $ \alpha $ to $\mathcal{T'}$
%                     \FOR {each $message m \in C$}
%                         \STATE Add a tree leaf node to $\mathcal{T'}$
%                     \ENDFOR 
%                 \ENDFOR 
%                 \STATE $P'$ $\leftarrow$  run vanilla 2D SE minimization with the initial encoding tree set to $\mathcal{T'}$
%             \ENDFOR 

%             \IF {$|V'|$ = 1}
%                 \STATE Break
%             \ENDIF
%             \IF {$P$ is the same as at the end of the last iteration}
%                 \STATE $n = 2n$
%             \ENDIF
%         \ENDWHILE

%         \RETURN $P$
%     \end{algorithmic}
% \end{algorithm}
% }
